# Supplementary material for: Emergence of Compositional Language with Deep Generational Transmission
Source: arXiv:1904.09067 source file (2020-05-27)
Supplement: Supplementary file 1 [file model_details.tex]

\begin{figure}[h]
\centering
\resizebox{0.85\columnwidth}{!}{\large\begin{algorithm}[H]
\caption{Training with \textcolor{blue}{Replacement} and \textcolor{red}{Multiple Agents}}
\label{alg:train_aug}
\For{epoch $e=1, \ldots, N_{\text{epochs}}$}{
    \textcolor{red}{Sample $\min{N_Q, N_A}$ bot pairs without replacement to form list $P$ of bot pairs.}
    \For{each bot pair $i_Q, i_A$ in $P$}{
        \For{each batch $x_Q, x_A, u$}{
            \For{dialog rounds $t=1,\ \ldots \ ,T$}{
                $m_Q^t, v_Q^t, h_Q^t = Q^{i_Q}(m_A^{t-1}, x_Q, h_Q^{t-1})$ \\
                $m_A^t, v_A^t, h_A^t = A^{i_A}(m_Q^{t-1}, x_A, h_A^{t-1})$ \\
            }
            $\hat{u}^1, v_U^1, \hat{u}^2, v_U^2 = U^{i_Q}(x_Q, h_Q^T)$ \\
            $R = \ind{(u^1 = \hat{u}^1) \wedge (u^2 = \hat{u}^2)}$ \\
            $\mathcal{L}_Q =
             \sum_{i=1}^2 \left[
                (v_U^i - R)^2 - (R - \bot\footnotemark( v_U^i ))\log p(\hat{u}^i) 
             \right] + $ \\
            \hspace{28pt}
            $\sum_{t=1}^2 \left[
                (v_Q^t - R)^2 - (R - \bot( v_Q^t ))\log p(m_Q^t)
             \right]$ \\
            Gradient update of \qbot{} $i_Q$ using $\mathcal{L}_Q$ \\
            $\mathcal{L}_A =
             \sum_{t=1}^2 \left[
                (v_A^t - R)^2 - (R - \bot( v_A^t ))\log p(m_A^t)
             \right]$ \\
            Gradient update of \abot{} $i_A$ using $\mathcal{L}_Q$ \\
        }
    }
    \textcolor{blue}{
    \If{$e~\mathrm{mod}~E = 0$}{
        Sample replacement set $B$ under policy $\pi$ and
        re-initialize all agents in $B$
    }}
}
\Return all \qbot{}s and \abot{}s.
\end{algorithm}}
\end{figure}
\footnotetext{Here $\bot(\cdot)$ is the stop gradient operator.}
